# Supplementary material for: MagicAgent: Towards Generalized Agent Planning
Source: arXiv:2602.19000 source file (2026-03-01)
Supplement: Supplementary file 1 [file demo_bak.tex]

\newtcolorbox{promptbox}[1]{
    colback=gray!10,        % 主体浅灰色背景
    colframe=black,         % 外边框黑色
    boxrule=1pt,            % 边框粗细
    arc=5pt,                % 圆角半径
    left=0pt, right=0pt,    % 内部左右边距清零，方便黑条铺满
    top=0pt, bottom=5pt,    % 底部留一点空隙
    % breakable,              % <--- 加入这一行核心代码
    enhanced,               % 建议加上这个，效果更好
    title=#1,
    fonttitle=\bfseries\sffamily\Large,
    coltitle=white,
    colbacktitle=black,     % 第一级标题黑底
    attach boxed title to top left={xshift=0mm, yshift=0mm},
    boxed title style={sharp corners, size=small, frame hidden}
}

\newcommand{\sectionbar}[1]{
    \begin{tcolorbox}[
        colback=black!85, 
        colframe=black!85,
        sharp corners,
        left=6pt,
        right=6pt,
        top=3pt,
        bottom=2pt,
        grow to left by=0pt,
        grow to right by=0pt,
        boxrule=0pt
    ]
    % \textcolor{white}{\textbf{#1}}
    \textcolor{white}{\sffamily\bfseries\small #1}
    \end{tcolorbox}
}

\lstset{
    basicstyle=\small\ttfamily,
    columns=flexible,
    breaklines=true,
    showstringspaces=false,
    xleftmargin=20pt,
    lineskip=-0.5pt,
    upquote=true
}


\section{Hierarchical Task Decomposition Examples}
\label{td_examples}

Here are two examples in Hierarchical Task Decomposition.
\vspace{10pt}
\begin{promptbox}{}
    \sectionbar{Raw Format}
    \vspace{2pt}
    \begin{tcblisting}{
        % --- tcblisting 自身的样式，让它看起来“隐形”并融入外部盒子 ---
        sharp corners,          % 尖角，与外部容器匹配
        boxrule=0pt,            % 无边框
        frame hidden,
        colback=gray!10,
        colframe=gray!10,
        grow to left by=0pt,    % 左右紧贴外部容器
        grow to right by=0pt,
        top=0pt,                % 上下留出一点空白
        bottom=0pt,
        left=0pt,           % 左侧边距
        right=0pt,
        boxsep=1mm,
        listing only,
        listing options={
            % basicstyle=\ttfamily\small, % 字体大小，推荐 small
            basicstyle=\ttfamily\scriptsize\microtypesetup{activate=false},
            breaklines=true,            % 允许自动换行（对长中文很重要）
            columns=fullflexible,       % 紧凑排列
            xleftmargin=0pt,            % 【核心】强制代码左边距为0，完全由上面的 left=5pt 控制
            xrightmargin=0pt,
            aboveskip=0pt,              % 清除代码块上下的垂直额外间距
            belowskip=0pt,
            tabsize=2                   % 设置 Tab 为2个空格宽，避免 JSON 缩进过深
        }
    }
<Query>麻烦你去京东帮我清空购物车可以吗？</Query>\n<Plan>Step1. 在京东中清空购物车里的所有商品</Plan>\n<Reply>Plan完成</Reply>
    \end{tcblisting}
    \vspace{2pt}
    
    \sectionbar{OpenAI Format}

    \begin{tcblisting}{
        % --- tcblisting 自身的样式，让它看起来“隐形”并融入外部盒子 ---
        sharp corners,          % 尖角，与外部容器匹配
        boxrule=0pt,            % 无边框
        frame hidden,
        colback=gray!10,
        colframe=gray!10,
        grow to left by=0pt,    % 左右紧贴外部容器
        grow to right by=0pt,
        top=0pt,                % 上下留出一点空白
        bottom=0pt,
        left=0pt,           % 左侧边距
        right=0pt,
        boxsep=1mm,
        listing only,
        listing options={
            % basicstyle=\ttfamily\small, % 字体大小，推荐 small
            basicstyle=\ttfamily\scriptsize\microtypesetup{activate=false},
            breaklines=true,            % 允许自动换行（对长中文很重要）
            columns=fullflexible,       % 紧凑排列
            xleftmargin=0pt,            % 【核心】强制代码左边距为0，完全由上面的 left=5pt 控制
            xrightmargin=0pt,
            aboveskip=0pt,              % 清除代码块上下的垂直额外间距
            belowskip=0pt,
            tabsize=2                   % 设置 Tab 为2个空格宽，避免 JSON 缩进过深
        }
    }
{
  "messages": [
    {
      "role": "user",
      "content": "麻烦你去京东帮我清空购物车可以吗？"
    },
    {
      "role": "assistant",
      "content": "<Plan>Step1. 在京东中清空购物车里的所有商品</Plan>\n<Reply>Plan完成</Reply>"
    }
  ]
}
    \end{tcblisting}
\end{promptbox}
\vspace{10pt}
\begin{promptbox}{}
    \sectionbar{Raw Format}
    % \vspace{6pt}
    % {
    %     \scriptsize
    %     \ttfamily
    %     \raggedright
    %     \CJKsetecglue{}
    %     <Query>帮我在美团预订杭州西湖的酒店，入住11月5日，离店11月7日，要订两个房间，顺便查一查附近有没有好吃的餐馆。</Query>\textbackslash n<Plan>Step1. 在美团中预订位于杭州的西湖酒店，入住日期为11月5日，离店日期为11月7日，预定2个房间\textbackslash nStep2. 在美团中搜索西湖酒店附近的美食餐馆，并按好评排序</Plan>\textbackslash n<Reply>Plan完成</Reply>
    % }
    \begin{tcblisting}{
        % --- tcblisting 自身的样式，让它看起来“隐形”并融入外部盒子 ---
        sharp corners,          % 尖角，与外部容器匹配
        boxrule=0pt,            % 无边框
        frame hidden,
        colback=gray!10,
        colframe=gray!10,
        grow to left by=0pt,    % 左右紧贴外部容器
        grow to right by=0pt,
        top=0pt,                % 上下留出一点空白
        bottom=0pt,
        left=0pt,           % 左侧边距
        right=0pt,
        boxsep=1mm,
        listing only,
        listing options={
            % basicstyle=\ttfamily\small, % 字体大小，推荐 small
            basicstyle=\ttfamily\scriptsize\microtypesetup{activate=false},
            breaklines=true,            % 允许自动换行（对长中文很重要）
            columns=fullflexible,       % 紧凑排列
            xleftmargin=0pt,            % 【核心】强制代码左边距为0，完全由上面的 left=5pt 控制
            xrightmargin=0pt,
            aboveskip=0pt,              % 清除代码块上下的垂直额外间距
            belowskip=0pt,
            tabsize=2                   % 设置 Tab 为2个空格宽，避免 JSON 缩进过深
        }
    }
<Query>帮我在美团预订杭州西湖的酒店，入住11月5日，离店11月7日，要订两个房间，顺便查一查附近有没有好吃的餐馆。</Query>\n<Plan>Step1. 在美团中预订位于杭州的西湖酒店，入住日期为11月5日，离店日期为11月7日，预定2个房间\nStep2. 在美团中搜索西湖酒店附近的美食餐馆，并按好评排序</Plan>\n<Reply>Plan完成</Reply>
    \end{tcblisting}
    \vspace{2pt}
    \sectionbar{OpenAI Format}
    \begin{tcblisting}{
        % --- tcblisting 自身的样式，让它看起来“隐形”并融入外部盒子 ---
        sharp corners,          % 尖角，与外部容器匹配
        boxrule=0pt,            % 无边框
        frame hidden,
        colback=gray!10,
        colframe=gray!10,
        grow to left by=0pt,    % 左右紧贴外部容器
        grow to right by=0pt,
        top=0pt,                % 上下留出一点空白
        bottom=0pt,
        left=0pt,           % 左侧边距
        right=0pt,
        boxsep=1mm,
        listing only,
        listing options={
            basicstyle=\ttfamily\scriptsize\microtypesetup{activate=false},
            breaklines=true,            % 允许自动换行（对长中文很重要）
            columns=fullflexible,       % 紧凑排列
            xleftmargin=0pt,            % 【核心】强制代码左边距为0，完全由上面的 left=5pt 控制
            xrightmargin=0pt,
            aboveskip=0pt,              % 清除代码块上下的垂直额外间距
            belowskip=0pt,
            tabsize=2                   % 设置 Tab 为2个空格宽，避免 JSON 缩进过深
        }
    }
{
  "messages": [
    {
      "role": "user",
      "content": "帮我在美团预订杭州西湖的酒店，入住11月5日，离店11月7日，要订两个房间，顺便查一查附近有没有好吃的餐馆。"
    },
    {
      "role": "assistant",
      "content": "<Plan>Step1. 在美团中预订位于杭州的西湖酒店，入住日期为11月5日，离店日期为11月7日，预定2个房间\nStep2. 在美团中搜索西湖酒店附近的美食餐馆，并按好评排序</Plan>\n<Reply>Plan完成</Reply>"
    }
  ]
}
    \end{tcblisting}
\end{promptbox}




\section{Tool-Augmented Planning Examples}
\label{tc_examples}

\begin{promptbox}{}
    
    \sectionbar{OpenAI Format}
    \begin{tcblisting}{
        % --- tcblisting 自身的样式，让它看起来“隐形”并融入外部盒子 ---
        sharp corners,          % 尖角，与外部容器匹配
        boxrule=0pt,            % 无边框
        frame hidden,
        colback=gray!10,
        colframe=gray!10,
        grow to left by=0pt,    % 左右紧贴外部容器
        grow to right by=0pt,
        top=0pt,                % 上下留出一点空白
        bottom=0pt,
        left=0pt,           % 左侧边距
        right=0pt,
        boxsep=1mm,
        listing only,
        listing options={
            basicstyle=\ttfamily\scriptsize\microtypesetup{activate=false},
            breaklines=true,            % 允许自动换行（对长中文很重要）
            columns=fullflexible,       % 紧凑排列
            xleftmargin=0pt,            % 【核心】强制代码左边距为0，完全由上面的 left=5pt 控制
            xrightmargin=0pt,
            aboveskip=0pt,              % 清除代码块上下的垂直额外间距
            belowskip=0pt,
            tabsize=2                   % 设置 Tab 为2个空格宽，避免 JSON 缩进过深
        }
    }
{
  "messages": [
    {
      "role": "user",
      "content": "帮我在美团预订杭州西湖的酒店，入住11月5日，离店11月7日，要订两个房间，顺便查一查附近有没有好吃的餐馆。"
    },
    {
      "role": "assistant",
      "content": "<think>\n用户要求\"帮我在美团预订杭州西湖的酒店，入住11月5日，离店11月7日，要订两个房间，顺便查一查附近有没有好吃的餐馆。\"。首先需要在美团中预订位于杭州的西湖酒店，入住日期为11月5日，离店日期为11月7日，并预订2个房间。\n</think>\n<action>{'name': 'book_hotel', 'arguments': {'app': '美团', 'city_slot': '杭州', 'hotel_slot': '西湖酒店', 'check_in_date_slot': '11月5日', 'departure_date_slot': '11月7日', 'number_slot': '2', 'payment_method_slot': '', 'filter_detail_slot': ''}}</action>"
    },
    {
      "role": "user",
      "content": "<observation>{'status': 'success', 'message': '酒店预订已成功提交，订单已生成，等待用户确认支付。', 'tool_result': {'booking_id': 'MT20241105001', 'hotel_name': '西湖酒店', 'city': '杭州', 'check_in_date': '2024-11-05', 'departure_date': '2024-11-07', 'room_count': 2, 'payment_method': '', 'total_price': 1680.0, 'reservation_status': '预定成功', 'additional_info': '已为您预留2间房，建议尽快完成支付以确保房间锁定。'}}</observation>"
    },
    {
      "role": "assistant",
      "content": "<think>\n用户要求\"帮我在美团预订杭州西湖的酒店，入住11月5日，离店11月7日，要订两个房间，顺便查一查附近有没有好吃的餐馆。\"。前一个步骤已经在美团中预订了位于杭州的西湖酒店，入住日期为11月5日，离店日期为11月7日，并预订2个房间。现在需要执行第二个步骤：在美团中搜索西湖酒店附近的美食餐馆，并按好评从好到坏进行排序。\n</think>\n<action>{'name': 'search_location', 'arguments': {'app': '美团', 'search_info_slot': '西湖酒店附近的餐馆', 'order_type': '按好评从好到坏排序'}}</action>"
    },
    {
      "role": "user",
      "content": "<observation>{'status': 'success', 'message': '已根据好评排序为您在美团搜索西湖酒店附近的餐馆，以下为推荐结果。', 'tool_result': [{'name': '湖畔人家餐厅', 'address': '西湖酒店旁湖滨路88号', 'distance': '120米', 'rating': 4.9, 'price': '人均¥120', 'popularity': 950, 'open_hours': '10:00-22:00', 'contact': '0571-88888888', 'extra_info': '主打杭帮菜，环境优雅'}, {'name': '西湖味道私房菜', 'address': '西湖酒店对面西湖路102号', 'distance': '200米', 'rating': 4.8, 'price': '人均¥98', 'popularity': 870, 'open_hours': '11:00-21:30', 'contact': '0571-87654321', 'extra_info': '特色菜品丰富，适合家庭聚餐'}, {'name': '绿茶餐厅（西湖店）', 'address': '西湖酒店附近南山路66号', 'distance': '350米', 'rating': 4.7, 'price': '人均¥85', 'popularity': 820, 'open_hours': '09:30-22:00', 'contact': '0571-81234567', 'extra_info': '环境舒适，适合朋友聚会'}]}</observation>"
    },
    {
      "role": "assistant",
      "content": "<think>\n当前已经完成用户任务要求，已在美团中预订了位于杭州的西湖酒店，入住日期为11月5日，离店日期为11月7日，并完成了2个房间的预订，同时已经查询并获取了西湖酒店附近的美食餐馆且按好评从好到坏进行了排序。\n</think>\n<action>{'name': 'finish', 'arguments': {'content': '已成功为您在美团预订了杭州西湖的酒店，酒店名称为“西湖酒店”，入住时间为2024年11月5日，离店时间为2024年11月7日，共预订了2间房，总价格为1680元，目前预订已成功，建议您尽快支付。此外，还根据好评排序，为您推荐了西湖酒店附近的几家餐馆：  \n1. 湖畔人家餐厅，地址：西湖酒店旁湖滨路88号，距离酒店约120米，评分4.9，人均消费120元，环境优雅，主打杭帮菜，营业时间10:00-22:00，联系电话：0571-88888888；  \n2. 西湖味道私房菜，地址：西湖酒店对面西湖路102号，距离酒店约200米，评分4.8，人均消费98元，菜品丰富，非常适合家庭聚餐，营业时间11:00-21:30，联系电话：0571-87654321；  \n3. 绿茶餐厅（西湖店），地址：西湖酒店附近南山路66号，距离酒店约350米，评分4.7，人均消费85元，环境舒适，适合朋友聚会，营业时间09:30-22:00，联系电话：0571-81234567。  \n\n您可以根据需求选择！'}}</action>"
    }
  ]
}
    \end{tcblisting}
\end{promptbox}



\section{Multi-Constraint Scheduling Examples}
\label{mcs_examples}

\begin{promptbox}{}
    \sectionbar{OpenAI Format}
    \begin{tcblisting}{
        % --- tcblisting 自身的样式，让它看起来“隐形”并融入外部盒子 ---
        sharp corners,          % 尖角，与外部容器匹配
        boxrule=0pt,            % 无边框
        frame hidden,
        colback=gray!10,
        colframe=gray!10,
        grow to left by=0pt,    % 左右紧贴外部容器
        grow to right by=0pt,
        top=0pt,                % 上下留出一点空白
        bottom=0pt,
        left=0pt,           % 左侧边距
        right=0pt,
        boxsep=1mm,
        listing only,
        listing options={
            basicstyle=\ttfamily\scriptsize\microtypesetup{activate=false},
            breaklines=true,            % 允许自动换行（对长中文很重要）
            columns=fullflexible,       % 紧凑排列
            xleftmargin=0pt,            % 【核心】强制代码左边距为0，完全由上面的 left=5pt 控制
            xrightmargin=0pt,
            aboveskip=0pt,              % 清除代码块上下的垂直额外间距
            belowskip=0pt,
            tabsize=2                   % 设置 Tab 为2个空格宽，避免 JSON 缩进过深
        }
    }
{
  "messages": [
    {
      "role": "user",
      "content": "You plan to visit 5 global cities for 25 days in total. You only take direct flights to commute between cities.You must be in Dubrovnik between day 15 and day 19 of your trip. You want to stay in Hamburg for 7 days. You want to stay in Nairobi for 6 days. You want to stay in Dubrovnik for 5 days. You want to stay in Vienna for 5 days. You want to stay in Miami for 6 days.\n\nHere are the cities that have direct flights:\nDubrovnik and Hamburg, Dubrovnik and Miami, Dubrovnik and Vienna, Nairobi and Miami, Vienna and Miami.\n\nFind a trip plan of visiting the cities for 25 days by taking direct flights to commute between them."
    },
    {
      "role": "assistant",
      "content": "Here is the trip plan for visiting the 5 European cities for 25 days:
          **Day 1-6:** Arriving in Nairobi and visit Nairobi for 6 days.
          **Day 6:** Fly from Nairobi to Miami.
          **Day 6-11:** Visit Miami for 6 days.
          **Day 11:** Fly from Miami to Vienna.
          **Day 11-15:** Visit Vienna for 5 days.
          **Day 15:** Fly from Vienna to Dubrovnik.
          **Day 15-19:** Visit Dubrovnik for 5 days.
          **Day 19:** Fly from Dubrovnik to Hamburg.
          **Day 19-25:** Visit Hamburg for 7 days."
    }
  ]
}
    \end{tcblisting}
\end{promptbox}

% \begin{promptbox}{Meeting planning}
%     \sectionbar{OpenAI Format}
%     \begin{tcblisting}{
%         % --- tcblisting 自身的样式，让它看起来“隐形”并融入外部盒子 ---
%         sharp corners,          % 尖角，与外部容器匹配
%         boxrule=0pt,            % 无边框
%         frame hidden,
%         colback=gray!10,
%         colframe=gray!10,
%         grow to left by=0pt,    % 左右紧贴外部容器
%         grow to right by=0pt,
%         top=0pt,                % 上下留出一点空白
%         bottom=0pt,
%         left=0pt,           % 左侧边距
%         right=0pt,
%         boxsep=1mm,
%         listing only,
%         listing options={
%             basicstyle=\ttfamily\scriptsize\microtypesetup{activate=false},
%             breaklines=true,            % 允许自动换行（对长中文很重要）
%             columns=fullflexible,       % 紧凑排列
%             xleftmargin=0pt,            % 【核心】强制代码左边距为0，完全由上面的 left=5pt 控制
%             xrightmargin=0pt,
%             aboveskip=0pt,              % 清除代码块上下的垂直额外间距
%             belowskip=0pt,
%             tabsize=2                   % 设置 Tab 为2个空格宽，避免 JSON 缩进过深
%         }
%     }
% {
%   "messages": [
%     {
%       "role": "user",
%       "content": "You are visiting Beijing for the day and want to meet as many friends as possible. Solve the problem by considering various different schedules and picking the best one to optimize your goals.\n\nTravel distances (in minutes):\n798 Art Zone to CBD: 45.\n798 Art Zone to Forbidden City: 49.\n798 Art Zone to Sanlitun: 16.\n798 Art Zone to Summer Palace: 7.\n798 Art Zone to Tiananmen Square: 16.\nCBD to 798 Art Zone: 40.\nCBD to Forbidden City: 59.\nCBD to Sanlitun: 57.\nCBD to Summer Palace: 52.\nCBD to Tiananmen Square: 54.\nForbidden City to 798 Art Zone: 17.\nForbidden City to CBD: 15.\nForbidden City to Sanlitun: 27.\nForbidden City to Summer Palace: 6.\nForbidden City to Tiananmen Square: 41.\nSanlitun to 798 Art Zone: 35.\nSanlitun to CBD: 22.\nSanlitun to Forbidden City: 18.\nSanlitun to Summer Palace: 27.\nSanlitun to Tiananmen Square: 60.\nSummer Palace to 798 Art Zone: 52.\nSummer Palace to CBD: 12.\nSummer Palace to Forbidden City: 28.\nSummer Palace to Sanlitun: 10.\nSummer Palace to Tiananmen Square: 5.\nTiananmen Square to 798 Art Zone: 7.\nTiananmen Square to CBD: 15.\nTiananmen Square to Forbidden City: 38.\nTiananmen Square to Sanlitun: 34.\nTiananmen Square to Summer Palace: 55.\n\nCONSTRAINTS: You arrive at Sanlitun at 07:15. Richard will be at 798 Art Zone from 13:15 to 15:01. You'd like to meet Richard for a minimum of 60 minutes. Donald will be at CBD from 11:00 to 13:01. You'd like to meet Donald for a minimum of 45 minutes. Abigail will be at Tiananmen Square from 08:30 to 12:25. You'd like to meet Abigail for a minimum of 30 minutes. Emma will be at Forbidden City from 12:15 to 13:42. You'd like to meet Emma for a minimum of 45 minutes. Nicholas will be at Summer Palace from 11:45 to 13:36. You'd like to meet Nicholas for a minimum of 60 minutes.\n\nYour response should start with 'SOLUTION:'."
%     },
%     {
%       "role": "assistant",
%       "content": "SOLUTION:You start at Sanlitun at 07:15. You travel to Tiananmen Square in 60 minutes and arrive at 08:15. You wait until 08:30. You meet Abigail for 30 minutes from 08:30 to 09:00. You travel to CBD in 15 minutes and arrive at 09:15. You wait until 11:00. You meet Donald for 45 minutes from 11:00 to 11:45. You travel to Forbidden City in 59 minutes and arrive at 12:44. You meet Emma for 45 minutes from 12:44 to 13:29. You travel to 798 Art Zone in 17 minutes and arrive at 13:46. You meet Richard for 60 minutes from 13:46 to 14:46."
%     }
%   ]
% }
%     \end{tcblisting}
% \end{promptbox}



% \begin{promptbox}{Calendar Scheduling}
%     \sectionbar{OpenAI Format}
%     \begin{tcblisting}{
%         % --- tcblisting 自身的样式，让它看起来“隐形”并融入外部盒子 ---
%         sharp corners,          % 尖角，与外部容器匹配
%         boxrule=0pt,            % 无边框
%         frame hidden,
%         colback=gray!10,
%         colframe=gray!10,
%         grow to left by=0pt,    % 左右紧贴外部容器
%         grow to right by=0pt,
%         top=0pt,                % 上下留出一点空白
%         bottom=0pt,
%         left=0pt,           % 左侧边距
%         right=0pt,
%         boxsep=1mm,
%         listing only,
%         listing options={
%             basicstyle=\ttfamily\scriptsize\microtypesetup{activate=false},
%             breaklines=true,            % 允许自动换行（对长中文很重要）
%             columns=fullflexible,       % 紧凑排列
%             xleftmargin=0pt,            % 【核心】强制代码左边距为0，完全由上面的 left=5pt 控制
%             xrightmargin=0pt,
%             aboveskip=0pt,              % 清除代码块上下的垂直额外间距
%             belowskip=0pt,
%             tabsize=2                   % 设置 Tab 为2个空格宽，避免 JSON 缩进过深
%         }
%     }
% {
%   "messages": [
%     {
%       "role": "user",
%       "content": "You are an expert at scheduling meetings. You are given a few constraints on the existing schedule of each participant, the meeting duration, and possibly some preferences on the meeting time. Note there exists a solution that works with existing schedule of every participant. Here are a few example tasks and solutions:\n\nTASK: You need to schedule a meeting for Amanda Junior, Richard Advisor for 60 between the work hours of 9:00 to 17:00 on Monday, Tuesday, Wednesday, Thursday, Friday.\n\nHere are the existing schedules for everyone during the days: \nAmanda Junior is busy on Monday during 09:00 to 09:30, 10:00 to 11:30, 12:00 to 14:00, 15:00 to 15:30, Tuesday during 09:00 to 09:30, 11:00 to 11:30, 12:00 to 14:00, 15:00 to 16:30, Wednesday during 09:00 to 09:30, 10:00 to 10:30, 11:00 to 11:30, 12:00 to 13:00, 13:30 to 14:30, 16:00 to 17:00, Thursday during 09:00 to 09:30, 10:00 to 12:30, 13:00 to 14:30, 15:00 to 15:30, 16:30 to 17:00, Friday during 09:00 to 09:30, 10:30 to 13:00, 13:30 to 14:30, 16:30 to 17:00; \nRichard Advisor is busy on Monday during 09:30 to 10:30, 11:30 to 12:00, 13:30 to 15:00, 15:30 to 17:00, Tuesday during 10:30 to 12:30, 13:00 to 15:00, 15:30 to 16:00, 16:30 to 17:00, Wednesday during 09:00 to 10:00, 10:30 to 11:00, 11:30 to 12:30, 13:00 to 13:30, 14:30 to 16:00, Thursday during 09:30 to 10:00, 10:30 to 11:00, 12:30 to 13:00, 14:00 to 15:00, 15:30 to 16:30, Friday during 09:30 to 10:30, 12:00 to 12:30, 13:00 to 13:30, 14:30 to 16:30\nAdditionally, please try to avoid scheduling the meeting between 11:00-12:00 on Thursday.\n\nThe group would like to meet at their earlist availability.\nFind a time that works for everyone's schedule and constraints. \nSOLUTION:"
%     },
%     {
%       "role": "assistant",
%       "content": "Here is the proposed time: Tuesday, 09:30 - 10:30 "
%     }
%   ]
% }
%     \end{tcblisting}
% \end{promptbox}


\section{Procedural Logic Orchestration Examples}
\label{plo_examples}

\begin{promptbox}{}
    \sectionbar{OpenAI Format}
    \begin{tcblisting}{
        % --- tcblisting 自身的样式，让它看起来“隐形”并融入外部盒子 ---
        sharp corners,          % 尖角，与外部容器匹配
        boxrule=0pt,            % 无边框
        frame hidden,
        colback=gray!10,
        colframe=gray!10,
        grow to left by=0pt,    % 左右紧贴外部容器
        grow to right by=0pt,
        top=0pt,                % 上下留出一点空白
        bottom=0pt,
        left=0pt,           % 左侧边距
        right=0pt,
        boxsep=1mm,
        listing only,
        listing options={
            basicstyle=\ttfamily\scriptsize\microtypesetup{activate=false},
            breaklines=true,            % 允许自动换行（对长中文很重要）
            columns=fullflexible,       % 紧凑排列
            xleftmargin=0pt,            % 【核心】强制代码左边距为0，完全由上面的 left=5pt 控制
            xrightmargin=0pt,
            aboveskip=0pt,              % 清除代码块上下的垂直额外间距
            belowskip=0pt,
            tabsize=2                   % 设置 Tab 为2个空格宽，避免 JSON 缩进过深
        }
    }
{
    "messages": [
        {
            "role": "system",
            "content": "You are a helpful task planner.\nFirst I will give you the task description and actions list you can take to finish the task, and your task is to plan a sequence of nodes which are subtasks to achieve the task. Each node of workflow is a subtask, and you can take actions to complete the subtask.\nAfter you construct the plan, since some subtasks may not be dependent on each other, while others may have dependencies, please convert these nodes of subtasks into a topology diagram based on the task relevance in the workflow. The Graph should start with START node, and end with END node. \nKeep your output in foramt:\nNode:\n1.{subtask_1}\n2.{subtask_2}\n...\nEdges:\n(START,1)\n...\n(n,END))"
        },
        {
            "role": "user",
            "content": "Here are two examples. You need to strictly follow the format provided in the examples.\nTask: In addition to the individual born in April 1963, what other artist did critics compare The Advent's energetic update of original techno to?\nThe api list you can use: ['Search for critical commentary comparing The Advent's energetic update of original techno to other artists.', 'Identify the individual born in April 1963 referenced in the question.', 'What is the primary purpose for which the Finnish Hound was bred?', 'Extract the name(s) of the artist(s) who were compared to The Advent by critics, excluding the individual identified in step 1.', 'Determine the specific city where this group was formed in 1968.']"
        },
        {
            "role": "assistant",
            "content": "Node:\n1: Identify the individual born in April 1963 referenced in the question.\n2: Search for critical commentary comparing The Advent's energetic update of original techno to other artists.\n3: Extract the name(s) of the artist(s) who were compared to The Advent by critics, excluding the individual identified in step 1.\nEdge: (START,1) (START,2) (1,3) (2,3) (3,END)"
        },
        {
            "role": "user",
            "content": "Task: when did the battle of antietam take place\nThe api list you can use: ['Identify which county in Nevada the Sheep Range is located.', 'Search for the Battle of Antietam to determine the exact date it occurred.', 'Identify a romantic comedy written by Habib Faisal.', 'What is the location (region, range, or district) of the Masherbrum mountain in Pakistan?']"
        },
        {
            "role": "assistant",
            "content": "Node:\n1: Search for the Battle of Antietam to determine the exact date it occurred.\nEdge: (START,1) (1,END)"
        },
        {
            "role": "user",
            "content": "Now it's your turn.\nTask: nearest metro station to salt lake city kolkata\nThe api list you can use: ['Search for the latest information on operational metro stations in Kolkata, especially in and around the Salt Lake City area.', 'Determine which specific district he represented in that period.', 'Determine the station(s) closest to the central part of Salt Lake City.', 'Identify which metro line covers Salt Lake City.']"
        },
        {
            "role": "assistant",
            "content": "Node:\n1: Search for the latest information on operational metro stations in Kolkata, especially in and around the Salt Lake City area.\n2: Identify which metro line covers Salt Lake City.\n3: Determine the station(s) closest to the central part of Salt Lake City.\nEdge: (START,1) (1,3) (1,2) (2,END) (3,END)"
        }
    ]
}
    \end{tcblisting}
\end{promptbox}

\section{Long-Horizon Tool Execution Examples}
\label{lhte_examples}

% \begin{promptbox}{Long-Horizon Tool Execution Trajectory}
%     \sectionbar{ShareGPT Format - Segment 1}
%     % --- 第一个代码块 ---
%     \begin{tcblisting}{
%         sharp corners,
%         boxrule=0pt,
%         frame hidden,
%         colback=gray!10,
%         colframe=gray!10,
%         grow to left by=0pt,
%         grow to right by=0pt,
%         top=0pt,
%         bottom=0pt,
%         left=0pt,
%         right=0pt,
%         boxsep=1mm,
%         breakable, % 既然已手动拆分，breakable 可留可不留，留着防万一
%         listing only,
%         listing options={
%             basicstyle=\ttfamily\scriptsize\microtypesetup{activate=false},
%             breaklines=true,
%             columns=fullflexible,
%             xleftmargin=0pt,
%             xrightmargin=0pt,
%             aboveskip=0pt,
%             belowskip=0pt,
%             tabsize=2
%         }
%     }
% {
%   "conversations": [
%     {
%       "from": "human",
%       "value": "Hello—can you help me cancel my flight and get a refund? I’m not going to make the trip anymore."
%     },
%     {
%       "from": "gpt",
%       "value": "I can help with that. Please provide your **user ID** and **reservation ID**. If you don’t know the reservation ID, tell me your user ID and I can look it up."
%     },
%     {
%       "from": "human",
%       "value": "My user ID is elena_park_2391. I don’t have the reservation number handy."
%     },
%     {
%       "from": "gpt",
%       "value": "<think>\nI need the user’s profile to locate their reservation IDs since they don’t have it. I will call the function get_user_details.\n</think>\n<tool_call>\n{\"name\": \"get_user_details\", \"arguments\": {\"user_id\": \"elena_park_2391\"}}\n</tool_call>\n"
%     },
%     {
%       "from": "human",
%       "value": "<observation>{\"user_id\":\"elena_park_2391\",\"email\":\"elena.park@email.com\",\"addresses\":[\"12 Waverly Pl, New York, NY\"],\"date_of_birth\":\"1990-11-14\",\"membership_level\":\"silver\",\"payment_methods\":[{\"payment_id\":\"credit_card_9047712\",\"type\":\"credit_card\"},{\"payment_id\":\"gift_card_1843995\",\"type\":\"gift_card\"}],\"reservation_numbers\":[\"QK3M7P\",\"L8V2RD\"]}</observation>"
%     },
%     {
%       "from": "gpt",
%       "value": "Thanks. I found two reservations on your profile: **QK3M7P** and **L8V2RD**. Which one would you like to cancel?"
%     },
%     {
%       "from": "human",
%       "value": "QK3M7P."
%     },
%     {
%       "from": "gpt",
%       "value": "<think>\nTo determine if cancellation/refund is allowed, I must check the reservation details (cabin, created_at within 24 hours, and whether any segment has been flown). I will call the function get_reservation_details.\n</think>\n<tool_call>\n{\"name\": \"get_reservation_details\", \"arguments\": {\"reservation_id\": \"QK3M7P\"}}\n</tool_call>\n"
%     },
%     {
%       "from": "human",
%       "value": "<observation>{\"reservation_id\":\"QK3M7P\",\"user_id\":\"elena_park_2391\",\"origin\":\"LGA\",\"destination\":\"ORD\",\"flight_type\":\"one_way\",\"cabin\":\"economy\",\"flights\":[{\"origin\":\"LGA\",\"destination\":\"ORD\",\"flight_number\":\"HAT312\",\"date\":\"2024-05-20\",\"price\":214}],\"passengers\":[{\"first_name\":\"Elena\",\"last_name\":\"Park\",\"dob\":\"1990-11-14\"}],\"payment_history\":[{\"payment_id\":\"credit_card_9047712\",\"amount\":214}],\"created_at\":\"2024-05-15T10:30:00\",\"total_baggages\":1,\"nonfree_baggages\":0,\"insurance\":\"no\"}</observation>"
%     },
%     {
%       "from": "gpt",
%       "value": "I can help cancel **QK3M7P** and process a refund because:\n- It’s **economy** (modifiable/cancellable if eligible),\n- The booking was created **2024-05-15 10:30 EST**, which is within **24 hours** of the current time (2024-05-15 15:00 EST),\n- No segment shows as already flown.\nBefore I proceed, please confirm:\n1) **Cancel reservation QK3M7P** (LGA → ORD, HAT312 on 2024-05-20) for **1 passenger (Elena Park)**\n2) Reason for cancellation: you said **change of plan**\n3) Refund will go back to the **original payment method (credit_card_9047712)** within **5–7 business days**\nReply **“yes”** to confirm and I’ll cancel it."
%     }
%     // ... (Content continues in the next block) ... 
%   ]
% }
%     \end{tcblisting}
% \end{promptbox}

% \begin{promptbox}{}
%     \sectionbar{ShareGPT Format - Segment 2}
%     % --- 第二个代码块 ---
%     \begin{tcblisting}{
%         sharp corners,
%         boxrule=0pt,
%         frame hidden,
%         colback=gray!10,
%         colframe=gray!10,
%         grow to left by=0pt,
%         grow to right by=0pt,
%         top=0pt,
%         bottom=0pt,
%         left=0pt,
%         right=0pt,
%         boxsep=1mm,
%         breakable, 
%         listing only,
%         listing options={
%             basicstyle=\ttfamily\scriptsize\microtypesetup{activate=false},
%             breaklines=true,
%             columns=fullflexible,
%             xleftmargin=0pt,
%             xrightmargin=0pt,
%             aboveskip=0pt,
%             belowskip=0pt,
%             tabsize=2
%         }
%     }
% {
%   "conversations": [
%     // ... (Continued from previous block) ...
    
%     {
%       "from": "human",
%       "value": "Yes, cancel it. Reason is change of plan."
%     },
%     {
%       "from": "gpt",
%       "value": "<think>\nUser confirmed cancellation and the reservation meets the 24-hour rule, with no flown segments. I will call the function cancel_reservation.\n</think>\n<tool_call>\n{\"name\": \"cancel_reservation\", \"arguments\": {\"reservation_id\": \"QK3M7P\"}}\n</tool_call>\n"
%     },
%     {
%       "from": "human",
%       "value": "<observation>{\"status\":\"cancelled\",\"reservation_id\":\"QK3M7P\"}</observation>"
%     },
%     {
%       "from": "gpt",
%       "value": "Done—reservation **QK3M7P** has been **cancelled**.\nYour refund will be issued back to the **original payment method (credit_card_9047712)** and should post within **5–7 business days**."
%     }
%   ],    
%   "domain": "Airline"
% }
%     \end{tcblisting}
% \end{promptbox}










\begin{promptbox}{}
    \sectionbar{ShareGPT Format}
    \begin{tcblisting}{
        sharp corners,          % 尖角，与外部容器匹配
        boxrule=0pt,            % 无边框
        frame hidden,
        colback=gray!10,        % 背景色与外部 promptbox 一致
        colframe=gray!10,
        grow to left by=0pt,    % 左右紧贴外部容器
        grow to right by=0pt,
        top=0pt,                % 上下留出一点空白
        bottom=0pt,
        left=0pt,           % 左侧边距
        right=0pt,
        boxsep=1mm,
        breakable,
        listing only,
        listing options={
            basicstyle=\ttfamily\scriptsize\microtypesetup{activate=false},
            breaklines=true,            % 允许自动换行（对长中文很重要）
            columns=fullflexible,       % 紧凑排列
            xleftmargin=0pt,            % 【核心】强制代码左边距为0，完全由上面的 left=5pt 控制
            xrightmargin=0pt,
            aboveskip=0pt,              % 清除代码块上下的垂直额外间距
            belowskip=0pt,
            tabsize=2,
            escapeinside={(*@}{@*)}
        }
    }
{
  "conversations": [
    {
      "from": "human",
      "value": "Hello—can you help me cancel my flight and get a refund? I’m not going to make the trip anymore."
    },
    {
      "from": "gpt",
      "value": "I can help with that. Please provide your **user ID** and **reservation ID**. If you don’t know the reservation ID, tell me your user ID and I can look it up."
    },
    {
      "from": "human",
      "value": "My user ID is elena_park_2391. I don’t have the reservation number handy."
    },
    {
      "from": "gpt",
      "value": "<think>\nI need the user’s profile to locate their reservation IDs since they don’t have it. I will call the function get_user_details.\n</think>\n<tool_call>\n{\"name\": \"get_user_details\", \"arguments\": {\"user_id\": \"elena_park_2391\"}}\n</tool_call>\n"
    },
    

    ---


    
        (*@\textcolor{gray}{\itshape // omitted for brevity ...}@*)


    
    ---

    
    {
      "from": "human",
      "value": "Yes, cancel it. Reason is change of plan."
    },
    {
      "from": "gpt",
      "value": "<think>\nUser confirmed cancellation and the reservation meets the 24-hour rule, with no flown segments. I will call the function cancel_reservation.\n</think>\n<tool_call>\n{\"name\": \"cancel_reservation\", \"arguments\": {\"reservation_id\": \"QK3M7P\"}}\n</tool_call>\n"
    },
    {
      "from": "human",
      "value": "<observation>{\"status\":\"cancelled\",\"reservation_id\":\"QK3M7P\"}</observation>"
    },
    {
      "from": "gpt",
      "value": "Done—reservation **QK3M7P** has been **cancelled**.\nYour refund will be issued back to the **original payment method (credit_card_9047712)** and should post within **5–7 business days**."
    }
  ],    
  "domain": "Airline"
}
    \end{tcblisting}
\end{promptbox}
